# Supplementary material for: Motion Similarity Modeling -- A State of the Art Report
Source: arXiv:2008.05872 source file (2020-08-13)
Supplement: Supplementary file 1 [file appendix.tex]

\appendix
\section*{Appendix}
%\appendixpage
%\addappheadtotoc

\begin{table}[h]
	\centering
		\begin{tabular}{c c c c p{1cm} c c c c }
			Glag. 						& \LaTeX 	& Class & ClassIdx	&	&	Glag. 						& \LaTeX 	& Class & ClassIdx\\
			\hline
			\glag{a} 					& a			& a					& 1 			& & \glag{n} 					& n			& n					& 17 \\
			\glag{b} 					& b			& b					& 2 			& & \glag{o} 					& o			& o					& 18 \\
			\glag{v}\sub{a} 	& v			& v\sub{a}	& 130 		& & \glag{p} 					& p			& p					& 19 \\
			\glag{v}\sub{b} 	& v			& v\sub{b}	& 131 		& & \glag{r} 					& r			& r					& 21 \\
			\glag{g} 					& g			& g					& 4 			& & \glag{s} 					& s			& s					& 22 \\
			\glag{d}\sub{a} 	& d			& d\sub{a}	& 150 		& & \glag{t} 					& t			& t					& 23 \\
			\glag{d}\sub{b} 	& d			& d\sub{b}	& 151 		& & \glag{u} 					& u			& ou				& 24 \\
			\glag{e} 					& e			& e					& 6 			& & \glag{f} 					& f			& f\_A			& 26 \\
			\glag{Zz}					& Zz		& zh				& 7 			& & \glag{h} 					& h			& kh				& 27 \\
			\glag{9}					& 9			& dz				& 8 			& & \glag{q} 					& q			& omega			& 29 \\
			\glag{z} 					& z			& z					& 9 			& & \glag{Ch}					& Ch		& sht				& 30 \\
			\glag{i} 					& i			& i\_A			& 10 			& & \glag{c} 					& c			& c					& 31 \\
			\glag{} 					&				& i\_B1 		& 11 			& & \glag{Cc}					& Cc		& ch				& 32 \\
			\glag{y} 					& y			& i\_B2			& 12 			& & \glag{Ss}					& Ss		& sh				& 33 \\
			\glag{j} 					& j			& gj				& 13 			& & \glag{4} 					& 4			& jor				& 34 \\
			\glag{k} 					& k			& k					& 14			& & \glag{7} 					& 7			& jer				& 38 \\
			\glag{l} 					& l			& l					& 15 			& & \glag{w} 					& w			& jat				& 39 \\
			\glag{m} 					& m			& m					& 16 			& & \glag{2} 					& 2			& ju				& 40 \\
		\end{tabular}
		\caption{Glagolitic alphabet with corresponding class labels and class indices.}
	\label{tab:latexLookup}
\end{table}
